# Supplementary material for: Electroluminescence from a polythiophene molecular wire suspended in a plasmonic scanning tunneling microscope junction
Source: arXiv:1401.2322 source file (2014-01-10)
Supplement: Supplementary file 1 [file Supplementary_information.pdf]

# Electroluminescence of a molecular wire suspended in a plasmonic junction.

Gaël Reecht, Fabrice Scheurer, Virginie Speisser,

Yannick J. Dappe, Fabrice Mathevet, Guillaume Schull

## CONTENTS

S1 – Dependency of the $\mathrm{d}I/\mathrm{d}V$ resonances with tip–sample distance. 2

S2 – Determining the energy dependency of the plasmon amplifications function $\Gamma(h\nu)$. 3

S3 – Tip–sample distance dependence of the plasmon modes. 4

S4 – Model for inelastic electron tunneling between molecular and metal states. 5

S5 – Energy of HOMO and LUMO states vs voltage. 7

S6 – Simulation of the $\mathrm{d}I/\mathrm{d}V$ spectra. 8

S7 – DFT simulations. 9

S8 – Impact of the wire conformation and of the wire length on the fluorescence. 10

References 12

**S1 – Dependency of the d$I$/d$V$ resonances with tip–sample distance.**

The d$I$/d$V$ spectra of figure 1c reveal essentially three resonances: a first resonance at $V \approx$ -0.8 V, another at $\approx$ 1.25 V, and a more intense resonance around 1.9 V. In the main text it is stated that the resonance at 1.25 V disappears when the tip is retracted, because of the decreasing current. To confirm this assertion we present in figure S1 d$I$/d$V$ spectra acquired for another wire junction for several tip–sample distances. Here, the progressive disappearance of the 1.25 V resonance is more clearly recognizable. These spectra also show that the position of the resonance at $\approx$ 1.9 V varies by $\approx$ 0.1 V in a non-monotonic manner with tip–sample distance. We attribute this effect to variations of the stress applied on the junction during the lifting procedure (i.e. a large (low) stress just before (after) detaching a thiophene unit from the surface) which affect the ratio between the voltage drop at the wire–substrate and wire–tip interfaces (referred further in the main manuscript as $Vd_s$ and $Vd_t$).

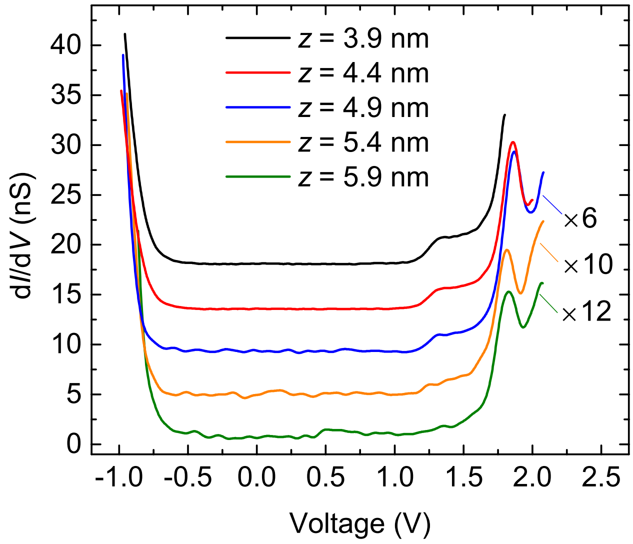


FIG. S1. Conductance d$I$/d$V$ spectra (lines) acquired at different tip–sample distances for a given polythiophene wire (the spectra are offseted for clarity).

## S2 – Determining the energy dependency of the plasmon amplifications function $\Gamma(h\nu)$.

It is now well established that STM induced light emission from noble metal electrodes is mediated by the coupling of inelastic tunnelling electrons traversing the junction with plasmons localized at the tip-sample cavity. In these experiments, the tip-sample cavity acts as a plasmonic nanoresonator exhibiting modes whose number and spectral shapes are intimately linked to the nanometer scale geometry of the tip apex [1]. These localized plasmons amplify any radiative transition occurring within the junction (Purcell effect) and affect the spectrum of the emitted light. To recover the intrinsic luminescence spectrum of an emitter located in a specific STM junction, it is therefore mandatory to correct for the energy dependency of the plasmon amplification function $\Gamma(h\nu)$ of the same STM junction. In the simple case of a pristine metallic junction, the number of emitted photons ($N(h\nu, V)$) follows [2]

$$N(h\nu, V) \propto \Gamma(h\nu) \int_{h\nu}^{eV} T(E, V, z) dE. \tag{1}$$

where $T(E, V, z) = \exp(-z\sqrt{\frac{4m}{\hbar^2}(2\Phi + eV - 2E)})$ is an energy dependent transmission probability for the tunnelling electrons, $\Phi = 4\,\text{eV}$ is the Au(111) work function, and $m$ the electron mass. It follows that

$$\Gamma(h\nu) \propto \frac{N(h\nu, V)}{\int_{h\nu}^{eV} T(E, V, z) dE}. \tag{2}$$

For each experimental set $N(h\nu, V)$ is determined by recording an optical spectra acquired with a pristine junction at $V = 3$ V. Indeed, between $0 < V < 3$ V the density of electronic states of tip and sample is assumed constant and does not impact the shape of the recorded spectra. $\Gamma(h\nu)$ is then determined following expression (2).

### S3 – Tip–sample distance dependence of the plasmon modes.

Figure S2 shows two examples of optical spectra of suspended wire junction acquired at tip-sample distances of (a) $z = 4\,\mathrm{nm}$ and (b) $z = 5\,\mathrm{nm}$ together with their associated $\Gamma(h\nu)$. Note that the spectra in (a) were acquired with another STM tip than the spectra in (b) which explains the different spectral shape between these two data set. However, in both cases, the plasmon modes appear at nearly the same energies in $\Gamma(h\nu)$ and in the wire junction spectra (dashed lines). This systematically reproduced effect is rather surprising since, according to previous experimental [3] and theoretical works [4], a blue shift of the plasmon resonances with increasing $z$ is expected. For distances as large as 5 nm, the wavelength shift of the modes may be of several tens of nanometers [4]. How can one explain the absence of such a shift in our experiments? Recently, quantum tunnelling of plasmon modes was evidenced between two close-to-contact gold nanospheres acting as plasmon resonators [5]. This effect is observed for a sphere-sphere distance of $z \lesssim 0.5\,\mathrm{nm}$ and is mediated by tunnelling charge transfer across the junction. This effect leads to a reduced blue shift of the plasmon modes compared to what is expected from classical theory. Despite the much larger $z$ in our experiments, charge transport between tip and sample still occurs via the wire states. We speculate that these conductance channels act as pathways for plasmon tunnelling between tip and sample, leading to a reduction of the plasmon mode blue-shift with $z$.

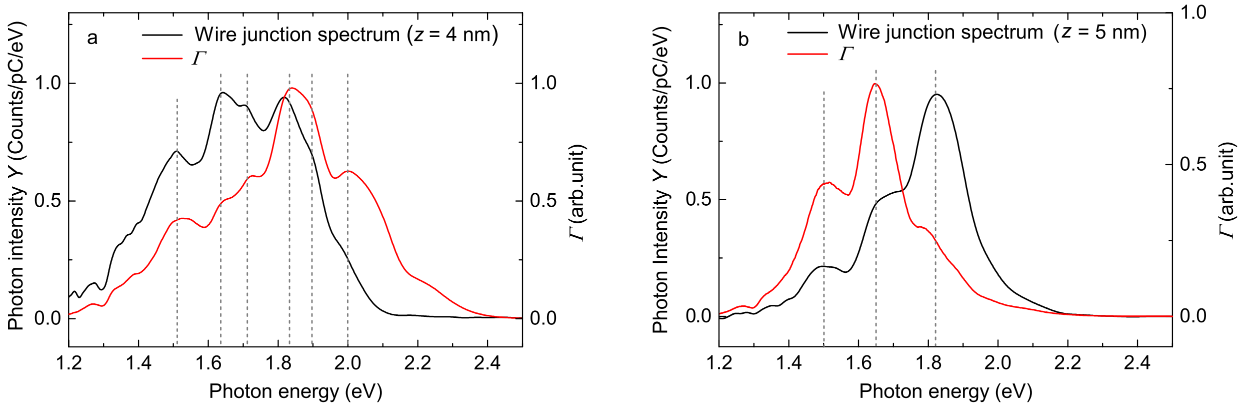


FIG. S2. Light emission spectra (black lines) of two typical wire junctions and their corresponding plasmon amplification functions $\Gamma(h\nu)$ (red lines). As indicated by the vertical dashed lines, the plasmon resonances are observed in both types of spectra at approximately the same energies.

## S4 – Model for inelastic electron tunneling between molecular and metal states.

Inelastic electron transition from the occupied states of one electrode to a molecular state (Fig. S3 a to c) or from a molecular state to the unoccupied state of an electrode (Fig. S3 d to f) are common light emission mechanisms reported for molecules directly adsorbed on a metal surface and probed with a metallic tip in the tunneling regime [2, 6]. For these mechanisms, the plasmon corrected spectra can be efficiently simulated [2] by considering that the number of emitted photons ($N$) scales with the available inelastic transitions for electrons starting from the occupied states of the tip and arriving in the HOMO of the molecule (3) or starting from the LUMO of the molecule and arriving in the unoccupied states of the sample (4)

$$N(h\nu, eV) \propto \int_{h\nu}^{eV} f_H(E - h\nu)\, dE, \quad \text{for } V > 0, \tag{3}$$

$$N(h\nu, eV) \propto \int_{h\nu}^{eV} f_L(E)\, dE, \quad \text{for } V > 0, \tag{4}$$

where $f_L$ and $f_H$ are Gaussian functions representing the LUMO and HOMO states (see manuscript for details).

Out of resonance, the intensity of the electronic waves in the wire decrease extremely fast with the distance from the electrodes. As a consequence, only inelastic transitions occuring in the close vicinity of the tip (sample) may efficiently contribute to the emission spectra in Fig. S3b (Fig. S3e). For these "close-to-electrode" transitions, the energy-dependent penetrability of the electronic waves in the junction is low. Its impact on the mecanisms depicted in Fig. S3b and e is neglectable and therefore disregarded in our simulations.

For $Vd_t/Vd_s$ = 1.5, $E_H$ = -0.6 eV and $E_L$ = 1.2 eV, the simulated optical spectra (Fig. S3 c and f) exhibit a shift of the high energy edge of the luminescence spectra with increasing bias and the formation of a "plateau" at low photon energy. None of these simulations reproduce the essential experimental findings, namely an emission peak whose maximum does not shift with voltage. Therefore, these two models must be disregarded.

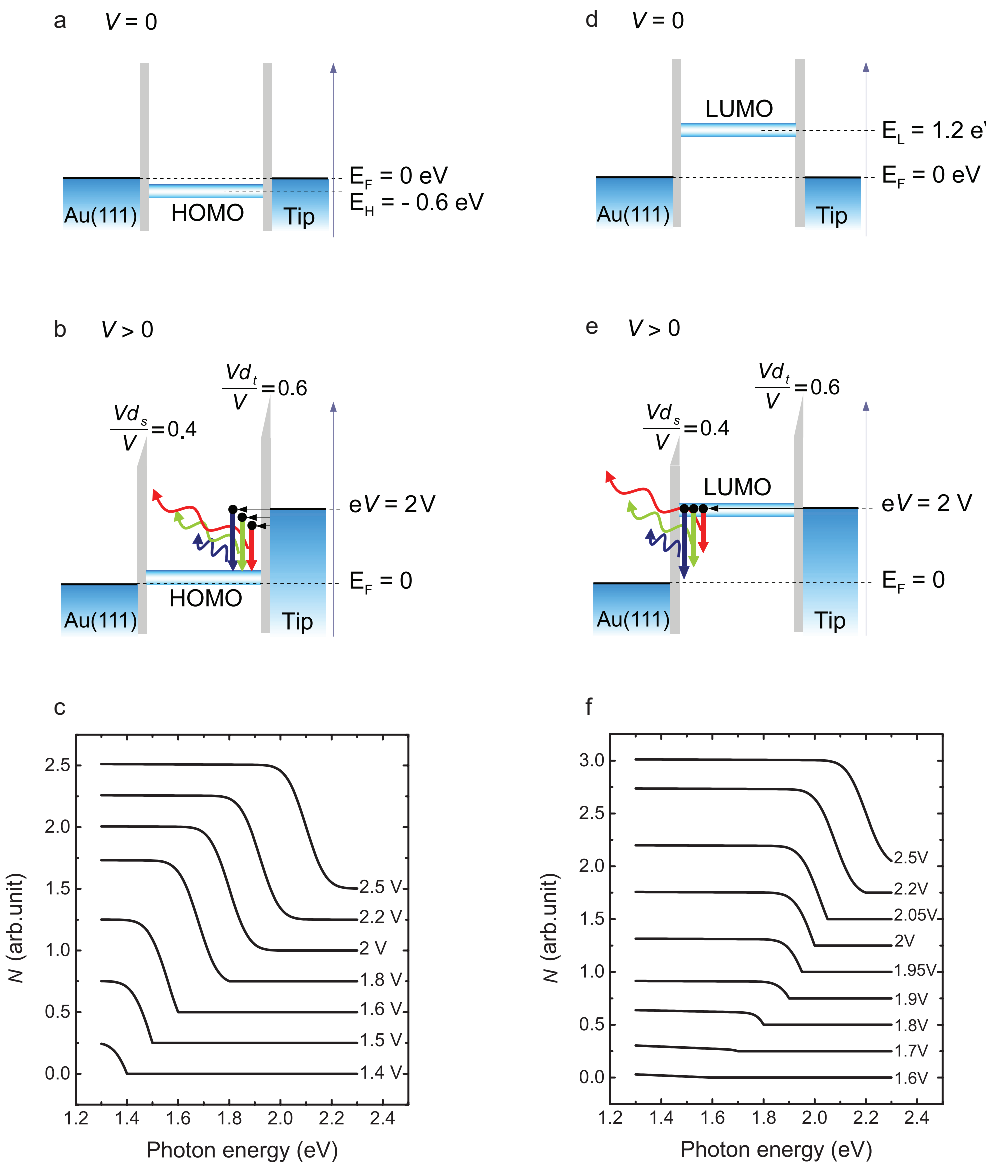


FIG. S3. Sketches of the models considering inelastic electron transitions from the occupied states of the tip to the HOMO of the suspended wire (a, b) and from the LUMO of the suspended wire to the unoccupied states of the sample (d, e), and the respective simulations (c) and (d) of the light emission spectra as a function of $V$.

## S5 – Energy of HOMO and LUMO states vs voltage.

Figure S4 shows how the energy of the peak maxima of the HOMO and LUMO derived orbitals of the wire evolves as a function of the applied voltage. For these plots, the Fermi level of the sample is set to zero and serves as a reference. The HOMO and LUMO energies ($E_H$ and $E_L$) at $V = 0$ and the respective voltage drops at each interfaces were chosen according to the procedure described in the main text. According to our model, radiative electronic transitions from the LUMO to HOMO may occur only when both states are between the Fermi level of the substrate and of the sample. These situations are highlighted in yellow in the plot of figure S4. Fluorescence onsets at $V \approx 2$ V and $V \approx$ -3 V can be deduced from these graphs. Experimentally, a fluorescence related emission is observed at a lower positive voltage ($V \approx 1.8$ V) because both HOMO and LUMO states have a non-zero bandwidth ($W \approx 0.15$ eV). The molecular junction could not stand high negative voltages without damages, and optical spectra could not be registrerd for $V < -1.6$ V. These plots illustrate and explain the observed polarity dependence of the wire junctions fluorescence.

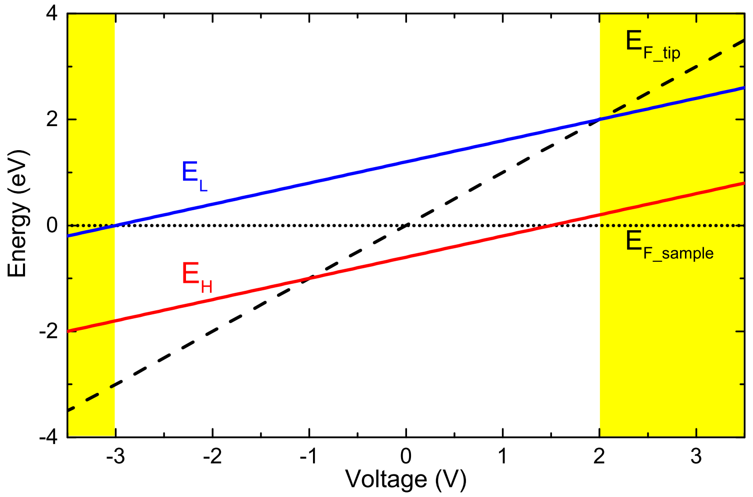


FIG. S4. Simulated voltage dependence of the energies of the HOMO ($E_H$) and LUMO ($E_L$) orbitals of the wire junction.

## S6 – Simulation of the d$I$/d$V$ spectra.

The simulation of the d$I$/d$V$ spectra is based on the sketches figure 3 a-c. The basic concept is that the current intensity $I$ rises when a molecular state crosses the Fermi level of the sample or of the tip. The d$I$/d$V$ spectra can then be approximated by

$$\frac{\mathrm{d}I(V)}{\mathrm{d}V} \propto \frac{\mathrm{d}}{\mathrm{d}V} \int_0^{eV} (f_L(E) + f_H(E))dE \,, \tag{5}$$

where $f_L$ and $f_H$ are Gaussian functions representing the LUMO and HOMO states (see main manuscript for details). The energy dependent transmission probabilities at the molecule–electrode interfaces (gray barriers in Fig. 3a-c) are neglected in this simulation.

## S7 – DFT simulations.

We have used Density Functional Theory (DFT) to modelise the suspended molecular junction. The equilibrium state and the energy minimum are determined using a very efficient DFT localized orbital molecular dynamics technique (FIREBALL) [7, 8]. Details on optimized numerical atomic orbital basis sets can be found elsewhere [9]. The considered geometry is a supercell of 6 × 6 Au atoms in the xy plane of four Au layers. On the top of this slab is set a "dodecathiophene", contacted with a model STM tip at one extremity and lying on the surface at the other. The STM tip is modelized by a pyramid of 4 Au atoms which is connected to a slab similar to the one used for the surface (Fig. S5a) in order to get an accurate description of the bulk electrons coming into the junction. For the relaxed configuration (Fig. S5a) the electronic transmission is calculated (Fig. S5b) using a non-equilibrium Keldysh-Green function formalism which takes multiple scattering into account [10, 11]. The spectrum in (Fig. S5b) is in good agreement with other simulations of closely related oligothiophene junctions [12].

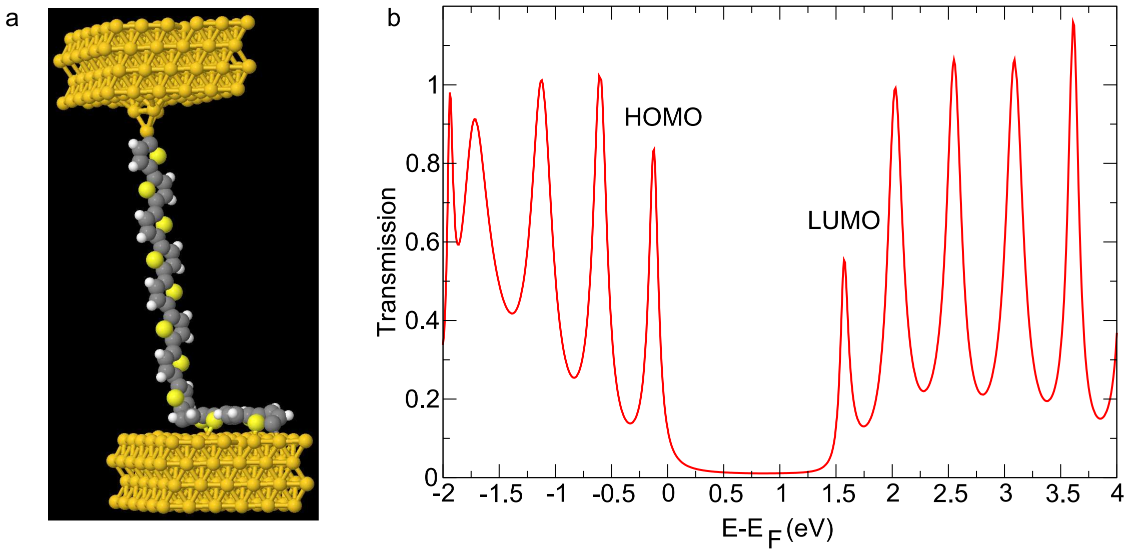


FIG. S5. (a) Geometry of the polythiophene junction as deduced from DFT simulations and (b) corresponding calculated transmission spectra.

**S8 – Impact of the wire conformation and of the wire length on the fluorescence.**

In Fig. S6 we compare, for a voltage of 1.8 V, the emission spectra of a same wire for different tip-sample distances. While the optical and $\mathrm{d}I/\mathrm{d}V$ spectra obtained for the two extreme tip excursions ($z = 3$ and 5 nm) are nearly identical, the situation is rather different for the intermediate distance ($z = 4.5$ nm). In this case substantial changes are observed in both the $\mathrm{d}I/\mathrm{d}V$ and the optical spectra, and are consistent with an increased HOMO – LUMO gap (Fig. S6d and e). We believe that the conformational changes caused by retracting the tip from $z = 3$ nm to $z = 4.5$ nm induced a stress on the suspended wire which changed the wire emission. Interestingly, when the tip was retracted further ($z = 5$ nm) the wire recovered its original properties, suggesting a stress release on the wire, probably provided by the detachment of one or several thiophene bases from the surface. The length of the suspended part of the wire has little influence on the energy of the emission or on the position of the $\mathrm{d}I/\mathrm{d}V$ resonances. This seems contradictory with the expected reduction of the optical gap with oligomer length. However, above 9 thiophene bases ($\approx$ 3 nm) the optical gap reduction with length is expected to be rather weak [13]. Moreover, the effective conjugation length is also affected by the part of the wire adsorbed on the surface and the coupling to the electrodes. We believe that these combined effects explain why no substantial changes of the emission energy or $\mathrm{d}I/\mathrm{d}V$ could be detected with $z$.

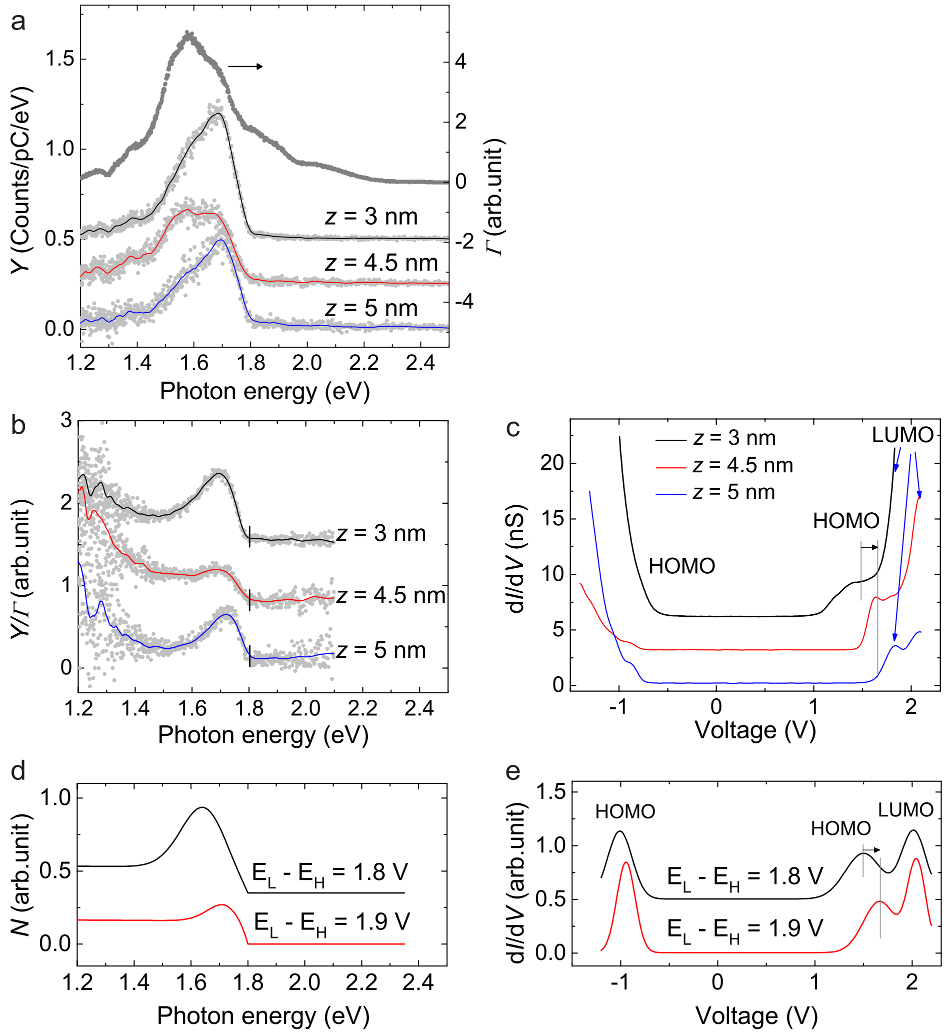


FIG. S6. (a) Raw and (b) plasmon–corrected optical spectra ($V = 1.8$ eV) of a same polythiophene junction for three tip–sample distances and (c) the corresponding d$I$/d$V$ spectra. The plasmon amplification function $\Gamma(h\nu)$ is shown (dots) in (a). Simulated optical (d) and d$I/dV$ (e) spectra according to the model described in the main text and for HOMO–LUMO gaps of 1.8 eV (black curves) and 1.9 eV (red curves). These plots illustrate the impact of the wire conformation on its optoelectronic properties.

[1] K. Meguro, K. Sakamoto, R. Arafune, M. Satoh, and S. Ushioda, Phys. Rev. B **65**, 165405 (2002).

[2] N. L. Schneider, F. Matino, G. Schull, S. Gabutti, M. Mayor, and R. Berndt, Phys. Rev. B **84**, 153403 (2011).

[3] J. Aizpurua, G. Hoffmann, S. P. Apell, and R. Berndt, Phys. Rev. Lett. **89**, 156803 (2002).

[4] I. Romero, J. Aizpurua, G. W. Bryant, and F. J. G. D. Abajo, Opt. Express **14**, 9988 (2006).

[5] K. J. Savage, M. M. Hawkeye, R. Esteban, A. G. Borisov, J. Aizpurua, and J. J. Baumberg, Nature **491**, 574 (2012).

[6] F. Geng, Y. Zhang, Y. Yu, Y. Kuang, Y. Liao, Z. Dong, and J. Hou, Opt. Express **20**, 26725 (2012).

[7] P. Jelínek, H. Wang, J. P. Lewis, O. F. Sankey, and J. Ortega, Phys. Rev. B **71**, 235101 (2005).

[8] J. P. Lewis, P. Jelínek, J. Ortega, A. A. Demkov, D. G. Trabada, B. Haycock, H. Wang, G. Adams, J. K. Tomfohr, E. Abad, H. Wang, and D. A. Drabold, Phys. Stat. Sol. B **248**, 1989 (2011).

[9] M. Basanta, Y. Dappe, P. Jelínek, and J. Ortega, Comput. Mater. Sci. **39**, 759 (2007).

[10] J. M. Blanco, C. González, P. Jelínek, J. Ortega, F. Flores, and R. Pérez, Phys. Rev. B **70**, 085405 (2004).

[11] G. Schull, Y. J. Dappe, C. González, H. Bulou, and R. Berndt, Nano Letters **11**, 3142 (2011).

[12] G. Peng, M. Strange, K. S. Thygesen, and M. Mavrikakis, J. Phys. Chem. C **113**, 20967 (2009).

[13] R. Telesca, H. Bolink, S. Yunoki, G. Hadziioannou, P. T. Van Duijnen, J. G. Snijders, H. T. Jonkman, and G. A. Sawatzky, Phys. Rev. B **63**, 155112 (2001).
